# Supplementary material for: Unsupervised Large Language Model Alignment for Information Retrieval via Contrastive Feedback
Source: arXiv:2309.17078 source file (2024-03-26)
Supplement: Supplementary file 1 [file Appendix.tex]

% \section{Prompt Template}
% \label{sec:prompt}

% \begin{table*}[]
% \caption{The templates used in our RLCF framework.}
% \label{tab:template}
% \begin{tabularx}{\linewidth}{lX}
% % \begin{tabular}{ll}
% \hline\hline
% \multicolumn{1}{l|}{Task}                                                                             & Template                                                                                                                     \\ \hline
% \multicolumn{2}{c}{Document Summarization}                                                                                                                                                                                           \\ \hline
% \multicolumn{1}{l|}{English Summarization}                                                                    & \begin{tabular}[c]{@{}l@{}}Please write a summarization for the document.\\ Document: \{d\}\\ Summarization:\end{tabular}\\ \hline
% \multicolumn{1}{l|}{Chinese Summarization}                                                                    & \begin{tabular}[c]{@{}l@{}}请为下面这个文档生成一个摘要:\\ 文档:\{d\}\\ 摘要:\end{tabular}                 \\ \hline
% \multicolumn{2}{c}{Data Augmentation}                                                                                                                                                                                                \\ \hline
% \multicolumn{1}{l|}{\begin{tabular}[c]{@{}l@{}}Passage Retrieval\&\\ Question Answering\end{tabular}} & \begin{tabular}[c]{@{}l@{}}Please write a question based on the document.\\ Document: \{d\_1\}\\ Question: \{q\_1\}\\ Document: \{d\_2\}\\ Question: \{q\_2\}\\ Document: \{d\}\\ Question:\end{tabular}                     \\ \hline
% \multicolumn{1}{l|}{Entity Retrieval}                                                                 & \begin{tabular}[c]{@{}l@{}}Please write a question about the main entity in the document.\\ Document: \{d\_1\}\\ Question: \{q\_1\}\\ Document: \{d\_2\}\\ Question: \{q\_2\}\\ Document: \{d\}\\ Question:\end{tabular}     \\ \hline
% \multicolumn{1}{l|}{Fact Checking}                                                                    & \begin{tabular}[c]{@{}l@{}}Please write a claim which could be supported/refuted by the passage.\\ Document: \{d\_1\}\\ Question: \{q\_1\}\\ Document: \{d\_2\}\\ Question: \{q\_2\}\\ Document: \{d\}\\ Question:\end{tabular} \\ \hline\hline
% \end{tabularx}
% \end{table*}



% The templates used in our RLCF framework are summarized in Figure~\ref{fig:templates} for reference.
% Each template begins with an instruction, outlining the tasks requirement of the LLMs.
% \begin{figure}
%     \centering
%     \includegraphics[width=\linewidth]{pics/templates.pdf}
%     \caption{The templates used in our RLCF framework.}
%     \label{fig:templates}
% \end{figure}

\begin{figure}
    \centering \includegraphics[width=0.7\linewidth]{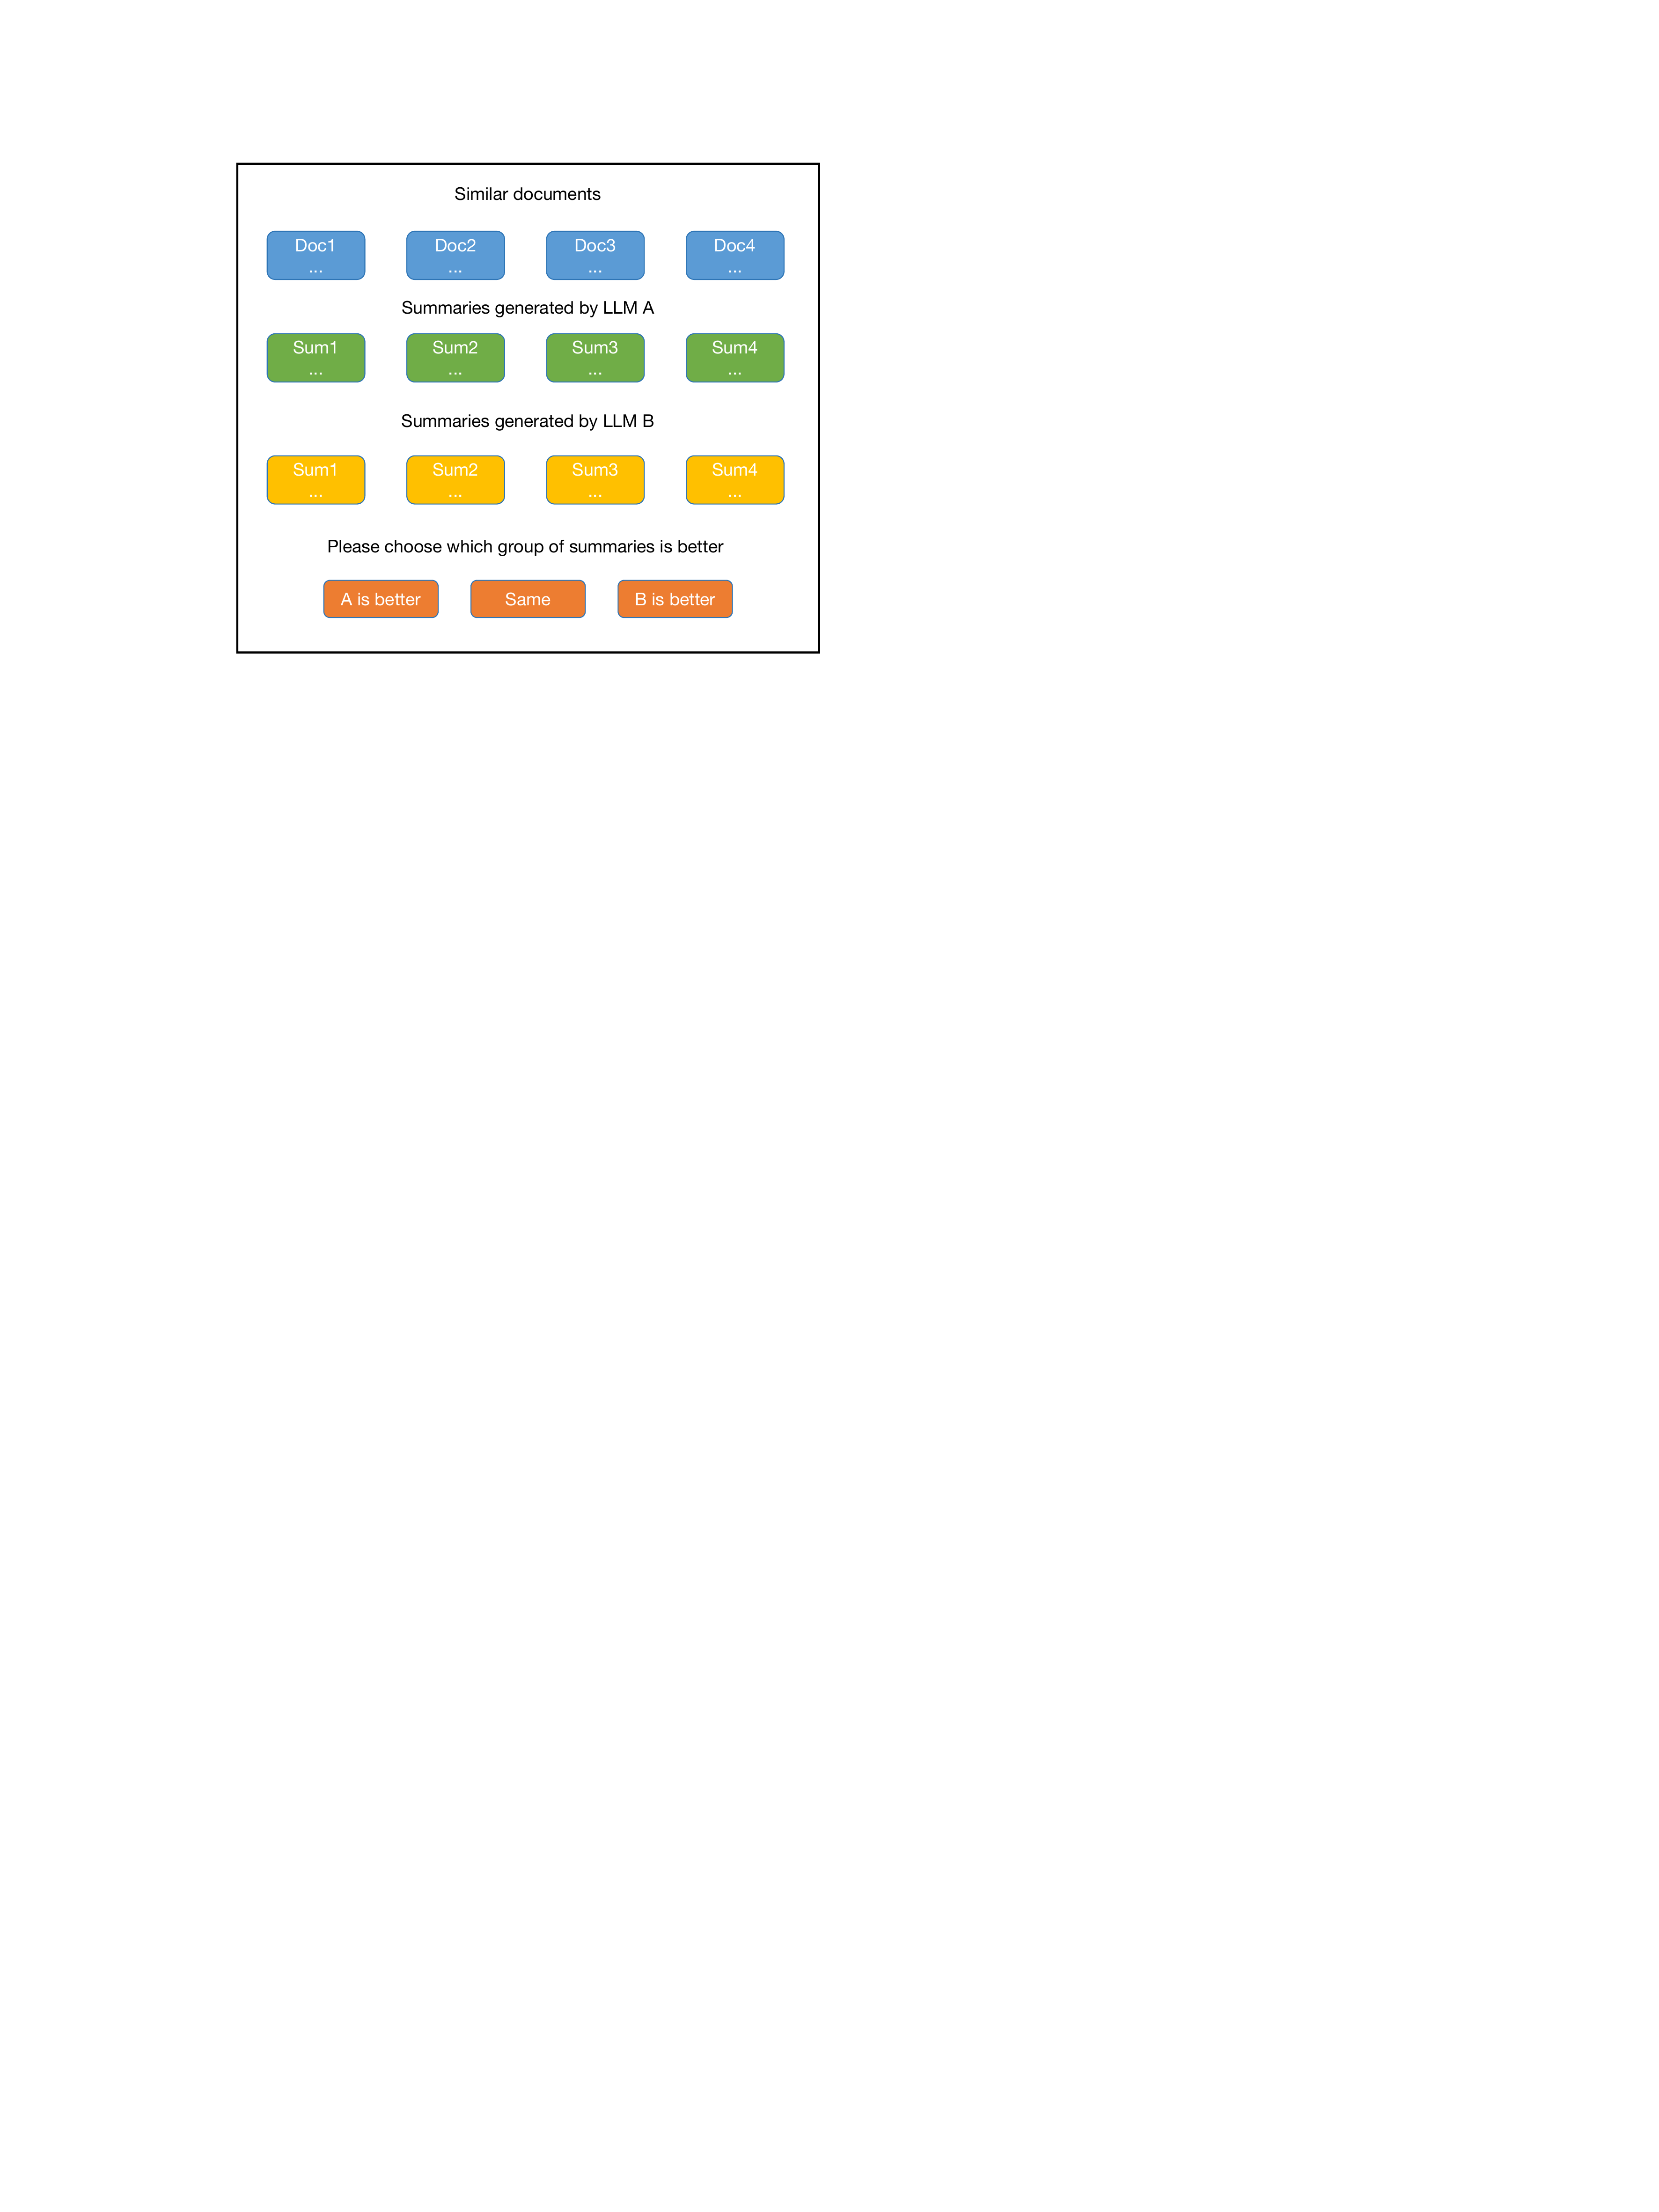}
    \caption{The illustration of annotation system.}
    \label{fig:annotationSys}
\end{figure}

\section{Annotation Guideline}
\label{sec:annotation}
The annotation guidelines involve three dimensions: distinctiveness, correctness and concision.
\begin{itemize}
    \item \textbf{Distinctiveness.} The concept of distinctiveness refers to the ability of the summary to distinguish itself from similar documents. It requires the summary to highlight unique and critical points that set it apart from other similar documents.
    % Can the summary be distinguished from similar documents?
    \item \textbf{Correctness.} 
    Correctness, in the context of a summary, entails the accuracy and completeness of the information presented. A correct summary faithfully represents the original content without distorting the meaning, omitting vital details, or introducing any inaccuracies. It should also cover all the essential points and arguments made in the original document, hence ensuring completeness.
    % Is the summary correct and complete?
    \item \textbf{Concision.} Concision concerns the brevity and succinctness of the summary. A concise summary effectively conveys the main points and arguments of the original document in as few words as possible, without losing critical information or context. It requires careful word choice and sentence construction to eliminate redundancy and verbosity.
    % Whether the summary is concise?
\end{itemize}

The annotation process in RLCF is conducted at the group level, wherein the ultimate decision regarding superior responses is made through comprehensive evaluation.
Annotation is conducted on the summaries produced by two distinct LLMs, i.e., RLCF-optimized LLM and the vanilla, unoptimized LLM. These two LLMs are randomly designated as LLM A and LLM B to avoid bias.
The annotator’s task is to assess the quality of the summaries and determine which one is superior. 
The decision is based on the above aspects of the summaries, i.e., distinctiveness, correctness, and concision.
% The labels of three-level annotation are presented in the following.
% \begin{itemize}
%     \item Label 0 denotes that summaries of LLM A are better to that of LLM B. 
%     \item Label 1 is assigned when the annotator deems that both summaries are of equal quality.
%     \item Label 2 denotes that summaries of LLM B are better to that of LLM A. 
% \end{itemize}
% \section{Case Study}
% \begin{table*}[]
% \caption{The cases of responses generated by vanilla LLMs and optimized LLMs for highly similar documents.}
% \label{table:case}
% \begin{tabularx}{\textwidth}{X|X|X|X}
% % \begin{tabular}{|l|c|l|l|l|l|l|l|l|}
% \hline\hline
% \multicolumn{4}{c}{Document summarization}\\\hline
% Documents                            & philippine share prices closed \#.\#\# percent lower thursday amid renewed fears about the global economic slowdown, dealers said. & philippine share prices closed \#.\#\# percent lower tuesday on fears that a congressional vote to quash an impeachment complaint against president gloria arroyo could lead to street protests and further political instability in the short-term,  dealers said. & philippine share prices closed \#.\#\# percent lower on tuesday, weighed down by the downturn in foreign markets, dealers said. \\ \hline
% Summaries generated by vanilla LLM   & philippine stocks close lower                                                                                                      & philippine stocks close lower                                                                                                                                                                                                                                       & philippine stocks close lower                                                                                                   \\ \hline
% Summaries generated by optimized LLM & philippine stocks close lower \textcolor{magenta}{amid global slowdown fears}                                                                           & philippine stocks close lower on \textcolor{magenta}{impeachment vote fears}                                                                                                                                                                                                             & philippine stocks close lower on \textcolor{magenta}{foreign market downturn}                                                                        \\ \hline
% \multicolumn{4}{c}{Query generation}\\\hline
% % \end{tabularx}
% % \end{table*}


% % \begin{table*}[]
% % \begin{tabularx}{\textwidth}{X|X|X|X}
% Documents                            & Shape based indexing for faster search of RNA family databases. BACKGROUND Most non-coding RNA families exert their function by means of a conserved, common secondary structure. The Rfam data base contains more than five hundred structurally annotated RNA families. Unfortunately, searching for new family members using covariance models (CMs) is very time consuming. & 
% % Hourly Forecast Detailed. 0am: The Anacortes, WA forecast for Apr 12 is 45 degrees and Patchy rain possible. 
% There is 74 percentage chance of rain and 8 mph \textcolor{red}{winds} from the North-Northeast. 3am: The Anacortes, WA forecast for Apr 12 is 44 degree sand Patchy rain possible. There is 75 percentage chance of rain and 7 mph \textcolor{red}{winds} from the North-Northeast. 6am:The Anacortes, WA forecast for Apr 12 is 44 degrees and Light rain. There is 79 percentage chance of rain and 5 mph \textcolor{red}{winds} from the East-Northeast, \textcolor{blue}{9am}: The Anacortes, WA forecast for Apr 12 is 48 degrees and Patchy light rain. & 0am: The Edmonds, WA forecast for Apr 12 is 46 degrees and Patchy rain possible. There is 76 percentage chance of rain and 5 mph \textcolor{red}{winds} from the Southwest. \textcolor{blue}{9am}: The Edmonds, WA forecast for Apr 12 is 43 degrees and Light rain. There is 80 percentage chance of rain and 6 mph \textcolor{red}{winds} from the East-Southeast. \\ \hline
% Queries generated by vanilla LLM   & What is the primary goal of the study?                                                                                                                                                                                                                                                                                                                                          & What is the temperature at \textcolor{blue}{9am}?                                                                                                                                                                                                                                                                                                                                                                                                                                                                                                                                                                        & What is the difference in the \textcolor{red}{wind} direction between the two times?                                                                                                                                                                                                                                              \\ \hline
% Queries generated by optimized LLM & How many \textcolor{magenta}{RNA} families are there in the \textcolor{magenta}{Rfam} database?                                                                                                                                                                                                                                           & Which time of day is it most likely to raining \textcolor{magenta}{Anacortes, WA}?                                                                                                                                                                                                                                                                                                                                                                                                                                                                                                                                          & Which time of the day is it expected to rain the most in \textcolor{magenta}{Edmonds}?                                                                                                                                                                                                                                                \\ \hline\hline
% \end{tabularx}
% \end{table*}
